# Supplementary material for: Data Analysis for a Balloon Borne Compton Polarimeter
Source: arXiv:2012.12939 source file (2020-12-23)
Supplement: Supplementary file 1 [file XSPEC.tex]

\large{XSPEC doc + Steps)
	\begin{itemize}
	\item Intro What is it?
	\item What we have?\\
		What we want out of it!
	\item Typical XSpec files. \\
		And our files (modified)
	\item How we generate these files. \\
	Tutorials here\\
	section subsection for each files 
	
	\item Arf
	\item Bins
	\item Normalization
	\item Binning -> Rebinning -> Grouping
	\end{itemize}
	
	\clearpage

	\section*{Appendix I: XSPEC}
	\addcontentsline{toc}{section}{Appendix I: XSpec}
	 XSPEC is a command line driven tool for spectral fitting by NASA.  It is part of 
	High Energy Astrophysics Software (HEAsoft) by High Energy Astrophysics Science Archive Research Center (HEASARC). It is widely used in the astrophysics and astronomy experiments for spectral fitting. XSpec also has specialized specific tools for few popular experiments like European X-Ray Observatory Satellite (EXOSAT), Chandra, etc. and quite a lot of generalized tools to deal with general experiments. Other HEAsoft tools like ftools and general commands can be used further to analyze and fit the data. (cite the manual or the page). 
	
	XSPEC can be used to spectral fit the observed GRAPE data. The processing of the GRAPE flight data results in an energy loss spectrum (column text file). The simulated mono-energetic runs is used to generate the response matrix and the effective area files (text files). PCA analysis on the flight data can be used to generate the background for each bins. Even though these are the ingredients for the spectral fitting, XSPEC only takes in certain file formats so we have to manipulate and convert these files into formats that XSPEC can read in. However, due to the lack of proper tutorials and documentation to understand this process, this Appendix section is created. \\
  	      
	\subsection*{XSPEC files}             
	             XSPEC requires the input files in the Flexible Image Transport System (FITS) files. Though we do not have any image data, we store the respective data in its extensions. A basic FITS file or its extension contains header and data. Header contains the information about the data and the various Using the commands and tools in XSPEC, FTOOLS and IDL (from Astronomical database package) we create, edit and manipulate the respective FITS file to be accepted by XSPEC. 
	             
	           \textbf{PHA files}    
	             
 		Pulse Height Analysis or the pha files are one of the mandatory files XSPEC requires. These have the .pha extensions attached to it. XSPEC requires them to be of OGIP standard format. There are few special formats for special missions that are accepted too. This information is included in the extension header. Typically these files contains the detector channels and the counts associated with it. The energy calibration and other supplementary information is included in additional extensions or in other files that are required by XSPEC to do the fits.               
		
		However, in our case we directly have an energy loss spectrum. Here we have energy channels but not the instrument channels information. The energy loss spectra is generated via processing the flight data. During processing various thresholds and filters are applied so this is generally the cleaner data that just needs to be spectral fit. IDL software is used to process and analyze the flight data and generate the energy loss spectrum in a form of text file. This text file contains four columns with lower energy bin value, higher energy bin value, counts and error in counts. Each row represents an energy bin and the counts and this is referred to as energy channel. The type of column with its name and units are stored in the respective extension headers so we have to be careful about it. We use a FTOOLS command named flx2xsp to generate a pha file which is a FITS file extension from the textfile. 
		
		\textbf{flx2xsp command}         
		
		This command, when executed, takes in a four column spectra text file and generates various files to be read in XSPEC. The name itself is flux to XSPEC file. So this procedure, without any modification is for looking at a photon spectra which is in a text format and analyzing it in XSPEC. This command generates two files. pha file and rsp file. The rsp file contains the ebounds and matrix extension which have the information of the energy bins and the response matrix. Since this is primarly a flux file, the response this creates is a diagonal one. For our case we have to modify this a little. The pha file contains the energy channels and counts information. The usage of this command is as follows:              
		
		$>$ flx2xsp infile phafile rspfile xunit yunit clobber

The infile is the input energy loss spectra file. The pha file and rsp file are respective pha and rsp files. The xunit defines the energy bin units (keV, MeV, etc) and y units (photons/s/cm2, etc).  The clobber overwrites the infile if present or else it will keep adding an extension. An example with this command and the pha file is present in the example section.

		\textbf{RSP files}        
		
		RSP files are another extension that is required by the XSPEC. This contains the information about the instrument response. Typically this contains two different extensions. Ebounds and Matrix extensions.                  
		
		Ebounds extensions contains the information about the energy channel bins. So it contains 3 columns, first is the energy channel number and the other two are energy low and energy high. These are similar as the energy loss spectrum text files first two columns. 
		Matrix extensions contains the information about the normalized response matrix. Understanding the formatting of the response matrix to the fits extension is challenging. There are not very clear documentation on the topic or proper examples to understand the format. My understanding of this topic is mainly based on the few documentations, a tool in XSPEC called dummyrsp and through few direct emails to the XSPEC help. The documentation that describes the most about the matrix extension is "The calibration required for the Spectral fit"
		%(https://heasarc.gsfc.nasa.gov/docs/heasarc/caldb/docs/memos/cal_gen_92_002/cal_gen_92_002.html). 
		The rsp file is a standard response file for the XSPEC which contains the redistribution matrix which is also called as the RMF file. 

%RMF Description Figures.	
	\input{Figures/appen_rmf_des}
	
	Looking at this table description was not enough to understand what each of the columns meant and how one would map the matrix elements to this format. Hence we ventured off on trying to find an example that would help us understand this better. We could not find a good example that helped us. However, we came across a tool called dummyrsp in  XSPEC that was partly helpful. This tool generated a dummy response matrix in the XSPEC for a use if needed and stored it in XSPEC cache. However, it did not create a separate rsp file. Moreover, there was no way of printing out the dummy rsp values which would help us understand more. The only word we had to take was form its documented description.
			
	A typical dummyrsp command would look like the following:                       
	  
	XSPEC12$>$ dummyrsp .0 30.0 3 lin 5.0 8.0                

	According to the description, this would create 3 incident channels from 0.0 to 30.0 that is linear. The offset of the detector energies is 5, which  means it starts from 5.0 and the bin is of 8.0 width. So the first detector bin is 5.0-13.0, and so forth. The number of detector channels depends on the range of incident energy channels. So, this would create the following response.            
	
	%Dummy Response	
	\input{Figures/appen_rmf_dummy}

	However there was no way to verify this easily. Since it did not create a rsp file, the question still remained on how to create an rsp file for a response similar to this. The  flx2xsp command generated a diagonal response so using this table and the diagonal response some of the column information was understood. The verification of these understandings were still in question so an email communication was made with the XSPEC contact and these queries were cleared. Since i wanted to clear my understanding of the rmf documentation, I presented the dummy matrix and showed how the dummy matrix values would be stored in an rsp file (describing the values in each rows and columns). It was verified that my understanding was correct. 
	
	So if i were to generate a response file for a response shown in Figure \ref{fig:appen_rmf_dummy}, My column values, according to the documentation shown in Figure \ref{fig:appen_rmf_des} would be as follows:          
% Figure of the rmf table understanding via the email.
	\input{Figures/appen_rmf_table}
	The channel numbers are energy channels for the detector that are in pha value and the energy range is specified in ebounds extension.                  
	
% EXAMPLE SECTION	
	\textbf{Walkthrough with an example}
	
	\textbf{Step 1: Spectra Text File}\\
	We begin with a text file of spectra called myspectra.txt. In our case this is generated after the flight data is processed, filtered and binned. Table  \ref{tab:appen_myspectra_table} shows an example of how this spectra file would look like. Each row represents an energy bin which are further referred to as energy channel. Hence this file contains 4 energy bins of size 8 each from 5.0 keV to 37.0 keV. 
	
	\begin{table}[H]
	\centering
	\begin{tabular}{l|l|l|l}
	Elow & Ehigh & Counts& Error \\ 
	\hline
	5.0 & 13.0 & 1.3 & 0.1 \\
	13.0 & 21.0 & 1.4 & 0.1 \\
	21.0  & 29.0 & 1.8 & 0.1 \\
	29.0 & 37.0 & 0.9 & 0.1 \\
	\end{tabular}
	\caption{Example of a textfile spectra: myspectra.txt (Note: the table lines are not presented in the textfile)}
	\label{tab:appen_myspectra_table}
	\end{table}	
	
	\textbf{Step 2: Generate the pha and rsp files}\\
	We use the  \textit{\textbf{flx2xsp}} command on this file to generate a rsp and a pha file by the following command: \\              
	$>\textit{\textbf{  flx2xsp myspectra.txt myspectra.pha myspectra.rsp clobber.}}$
	
	This command generates a pha extension fits file with the name \textit{myspectra.pha}. It also generates a rsp extension fits file with the name \textit{myspectra.rsp}. This filename is presented in the header of the pha file so in XSPEC when we load the pha file, the rsp file is automatically loaded. Additionally if we would like to associate this with a different rsp file, its better to edit the header in pha file. The rsp file has two extensions, ebounds and the matrix.       
	
	The \textbf{ebounds} extension contains the information about the detector energy channels. The data for ebounds has 3 columns twhich represents detector energy channel numbers, lower bin energy value and higher bin energy value. A data for the ebounds would be as follows: 
	
	\begin{table}[H]
	\centering
	\begin{tabular}{l|l|l}	
	Channel & Elow & EHigh\\
	\hline
	0& 0.5 & 13.0 \\
	\hline
	1& 13.0 & 21.0 \\
	\hline
	2 &21.0  & 29.0  \\
	\hline
	3 &29.0 & 37.0\\

	\end{tabular}
	\caption{Example of a ebounds extension for myspectra.txt data. Note that the column titles are stored in the header and not the column itself. }
	\label{tab:appen_ebounds}
	\end{table}
	
	This ebounds extension is already in the data format we want. Next we look at the matrix extension. The \textit{flx2xsp} command generated a diagonal response matrix for the matrix extension. This is not the data we want since our response matrix is non diagonal (triangular). So we have two options here, we can either re-write the data of the matrix extension or we create a new rsp file with the same ebounds extension, matrix extension header but  different matrix data. I preferred the latter since having a diagonal matrix might prove beneficial to do some sanity checks. 
		
	\textbf{Step 3: The new rsp file}\\	
	Our myspectra.rsp has 6 components to it. A header and data for primary, ebounds extension and matrix extension. We use readfits.pro in IDL to read in the header and data of the primary and create a new file named myresponse.rsp and write the same header and data in it. Secondly, we read and write the whole ebounds extension in it. With the response file we need to do a little more with it.                
	Firstly we use our simulations to generate a non-diagonal normalized (in probabilty) matrix and store it in a text file named myresponse.txt. Lets us assume our myresponse.txt has the following data which is basically the values of dummyrsp:       
	
		\begin{table}[H]
	\centering
	\begin{tabular}{l|l|l|l|l|l}
	Elow & Ehigh & DetChan1 & DetChan2 & DetChan3 &DetChan4\\
	\hline
	0.0& 10.0& 0.5 & 0 & 0 & 0 \\
	\hline
	10.0& 20.0 &0.3 &0.7 & 0 & 0 \\
	\hline
	20.0 &30.0  & 0.0 & 0.1 & 0.8 & 0.1 \\
	\end{tabular}
	\caption{myresponse.txt. Each row represents the incident mono-energetic energy and columns represent detector channel energies.}
	\label{tab:appen_myresponse.txt}
	\end{table}

	We define various structures in IDL in Figure \ref{fig:appen_rmf_des} and our understanding through email of these descriptions as shown in Figure \ref{fig:appen_rmf_table}. We then read in the text file and store the values in per line in the structures. So we would have a structure array as the length of the file (3 in this case) and each structure parameters define the columns. IDL does not support variable array so we have to define the max array length in some cases. Once we have read in the myresponse.txt into proper structures, the structure array is the data. We read in the myspectra.rsp header of the matrix extension, and write a matrix extension to myresponse.rsp with this header but the structured data. This will result in the response matrix we want for our XSPEC fit. 
	
	One final step would be edit a header in the pha file named RESPFILE that has the response file as myspectra.rsp and edit it to myresponse.rsp. Once we do this, we have the two basic files needed to do a spectral fit in XSPEC.
	\begin{itemize}
		
	\item Verify the command and the units. c/s vs photons/s/ cm2
		
	\item we need RMF file\\
	\item this has rsp file \\
			this has two extensions.
		and an arf file \\

	\end{itemize}
