# Supplementary material for: Data Analysis for a Balloon Borne Compton Polarimeter
Source: arXiv:2012.12939 source file (2020-12-23)
Supplement: Supplementary file 2 [file appen_specsheets.tex]

\chapter{Scintillator Specsheets}
\label{app:appen_specsheets}
%	\addcontentsline{toc}{chapter}{Appendix 1: Spec sheets}

 		%Figure
 	%Figure for Grape instrument e : another cartoon of the instrument array
\begin{figure}[hbtp]
 \centering
 	\includegraphics[width=0.95\textwidth]{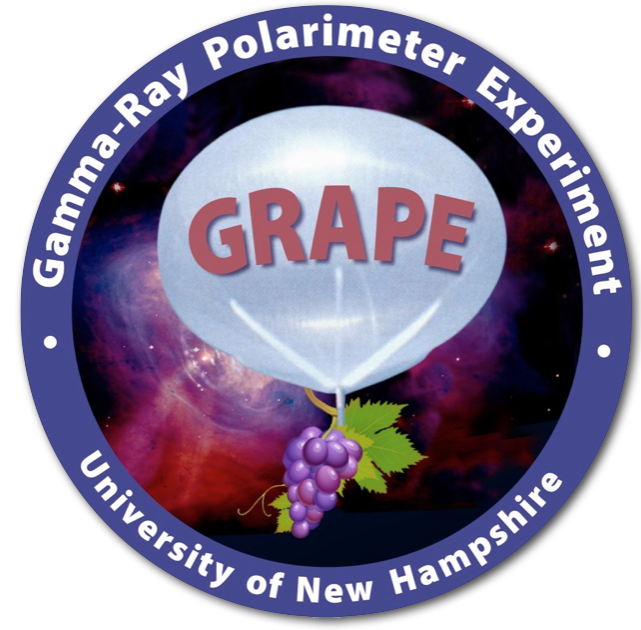}
    	\caption{Data sheet for calorimeter element}
    	\label{fig:cal_data_sheet}
\end{figure}		

%\begin{figure}[hbtp]
% \centering
%    	\includegraphics[width=0.95\textwidth]{cal_data_sheet_b}
%\end{figure}		 
		%Figure for Grape instrument e : another cartoon of the instrument array
\begin{figure}[hbtp]
 \centering
 	\includegraphics[width=0.95\textwidth]{grapelogo}
    	\caption{Data sheet for plastic element}
    	\label{fig:pla_data_sheet}
\end{figure}		

			%Figure for Grape instrument e : another cartoon of the instrument array
\begin{figure}[hbtp]
 \centering
	\includegraphics[width=0.95\textwidth]{grapelogo}
    	\caption{Data sheet for MAPMT}
    	\label{fig:mapmt_data_sheet}
\end{figure}		

%\begin{figure}[hbtp]
% \centering
    	%\includegraphics[width=0.95\textwidth]{cal_data_sheet_b}
	%	\includegraphics[width=0.95\textwidth]{grapelogo}
%\end{figure}		 
